# Supplementary material for: Learning Consistent Deep Generative Models from Sparse Data via Prediction Constraints
Source: arXiv:2012.06718 source file (2020-12-12)
Supplement: Supplementary file 1 [file supp_dataset_shar.tex]

\textbf{Overview.}
We consider a 9-way exclusive categorization task for the UniMiB SHAR dataset, classifying short recordings of 3-axis accelerometer data into the following possible categories: sitting up, lying down, standing up (from sitting), standing up (from lying down), walking, running, jumping, climbing up stairs, and climbing down stairs.

\textbf{Preprocessing}
We did \todo{FILL}

\textbf{Public availability.}
We will make code necessary to extract a similar dataset available after publication.

\paragraph{Data statistics.}
Statistics for SVHN are shown in Table~\ref{tab:svhn_stats}.

\begin{table}[!h]
\begin{tabular}{c c c}
split & num. examples & label distribution\\	
\midrule
labeled train & 16492 & 15.57
\\
unlabeled train & 16492 & 15.57
\\
labeled valid & 2007 & 15.35
\\
labeled test & 4582 & 15.33
\end{tabular}
\caption{SHAR dataset. \todo{FILL THIS TABLE}}
\label{tab:shar_stats}
\end{table}

\subsubsection{SHAR-Specific Experimental Settings}

\paragraph{Generative model.}

\paragraph{Prediction model.}

\paragraph{Hyperparameters.}
